# Supplementary material for: Contracting With a Reinforcement Learning Agent by Playing Trick or Treat
Source: arXiv:2410.13520 source file (2024-10-17)
Supplement: Supplementary file 1 [file appendix_honesty_old.tex]

\section{Omitted proofs from Section~\ref{sec:promise_form}}

\promiseFunctionsEq*
\begin{proof}	
	We prove the statement by induction over the steps $\mathcal{H}$ starting from $h = H$.
	For $h=H$, by the definitions of $\qprincipal_H(\tau,p,a)$ and $\qprincipalpr_H(s,\iota,p,a)$, it holds that:
	\begin{equation*}
		\qprincipal_H(\tau,p,a) = \sum_{\omega \in\Omega} F_H(\omega|s,a)r^P_H(s,\omega,p) = \qprincipalpr_H(s,\iota^\sigma_\tau,p,a)
	\end{equation*}
	for every history $\tau \in \mathcal{T}_H$ ending in state $s \in \mathcal{S}$, and couple $(p,a) \in \mathcal{X}$.
	Furthermore, since by construction $\varphi_H(p,a|s,\iota^\sigma_\tau) = \pi(p,a|\tau)$, it holds that:
	\begin{equation*}
		\vprincipal_H (\tau) = \sum_{(p,a) \in \mathcal{X}} \pi(p,a | \tau)  \qprincipal_H(\tau,p,a) = \sum_{(p,a) \in \mathcal{X}} \varphi_H(p,a|s,\iota^\sigma_\tau)  \qprincipalpr_H(s,\iota^\sigma_\tau,p,a) = \vprincipalpr_H(s,\iota^\sigma_\tau).
	\end{equation*}
	With a similar argument, it is possible to show that $\vagentpr_H (s,\iota^\sigma_\tau) = \vagent_H(\tau)$ and $\qagentpr_H(s,\iota^\sigma_\tau,p,a) = \qagent_H(\tau,p,a)$ for every state $s \in \mathcal{S}$, history $\tau \in \mathcal{T}_H$ ending in state $s$, and pair $(p,a) \in \mathcal{X}$.
	Furthermore, we observe that:
	\begin{equation*}
		\qagentdev_H(\tau,p,a) = \max_{\widehat{a} \in A} \sum_{\omega \in \Omega} F_H(\omega|s,\widehat{a}) r^P(s,\omega,p) = \qagentdevpr_H(s,\iota^\sigma_\tau,p,a).
	\end{equation*}
	Consequently:
	\begin{equation*}
		\vagentdev_H (\tau) = \sum_{(p,a) \in \mathcal{X}} \pi(p,a | \tau)  \qagentdev_H(\tau,p,a) = \sum_{(p,a) \in \mathcal{X}} \varphi_H(p,a|s,\iota^\sigma_\tau)  \qagentdevpr_H(s,\iota^\sigma_\tau,p,a) = \vagentdevpr_H(s,\iota^\sigma_\tau).
	\end{equation*}
	
	Now we consider a generic step $0<h<H$ and assume that the statement holds for $h+1$.
	For every history $\tau \in \mathcal{T}_h$, contract $p \in \mathcal{B}$ and action $a \in \A$, the following holds:
	\begin{equation*}
		\qprincipal_h(\tau,p,a) = \sum_{\omega \in \Omega}F_h(\omega|s,a) \left( r^\text{P}_h(s,\omega,p) + \sum_{s' \in \sset} P_h(s'|s,w)\vprincipal_{h+1}(\tau \oplus (a,\omega,s')) \right).
	\end{equation*}
	We observe that $\vprincipal_{h+1}(\tau \oplus (a,\omega,s')) = \vprincipalpr_{h+1}(s,\iota^\sigma_{\tau \oplus (a,\omega,s')})$ by inductive hypothesis.
	Furthermore, $\iota^\sigma_{\tau \oplus (a,\omega,s')} = g_h(s,a,\omega,\iota^\sigma_\tau,s')$ by construction (see Algorithm~\ref{alg:implement}).
	It follows that $\qprincipal_h(\tau,p,a) = \qprincipalpr_h(s,\iota^\sigma_\tau,p,a)$.
	As a further step, we observe that:
	\begin{equation*}
		\vprincipal_h (\tau) = \sum_{(p,a) \in \mathcal{X}} \pi(p,a | \tau)  \qprincipal_h(\tau,p,a) = \sum_{(p,a) \in \mathcal{X}} \varphi_H(p,a|s,\iota^\sigma_\tau)  \qprincipalpr_H(s,\iota^\sigma_\tau,p,a) = \vprincipalpr_H(s,\iota^\sigma_\tau).
	\end{equation*}
	A similar argument shows that the statement holds for the agent's value and action-value functions, concluding the proof.
\end{proof}

\honestyValue*
\begin{proof}
	We prove the statement by induction over the time steps $h \in \mathcal{H}$, starting from $h=H$.
	When $h=H$, for every state $s \in \mathcal{S}$, promise $\iota \in I_H(s)$ and couple $(p,a) \in \mathcal{X}$ such that $\varphi_H(p,a|s,\iota)>0$ the following holds:
	\begin{equation*}
		\qagentpr_H(s,\iota,p,a) = \sum_{\omega \in \Omega} F_H(\omega|s,a)r^A_H(s,\omega,p,a) \ge q_H(s,\iota,a) - \eta,
	\end{equation*}
	where the equality holds by definition of $\qagentpr_H(s,\iota,p,a)$, while the inequality holds because $\sigma$ is $\eta$-persuasive.
	Thus, by considering he definition of $\vagentpr_H(s,\iota)$, we have that:
	\begin{align*}
		\vagentpr_H(s,\iota) &= \sum_{(p,a) \in \mathcal{X}} \varphi_H(p,a|s,\iota) \qagentpr_H(s,\iota,p,a) \\
		&\ge \sum_{(p,a) \in \mathcal{X}} \varphi_H(p,a|s,\iota) (q_H(s,\iota,a) - \eta) \\
		&= \sum_{(p,a) \in \mathcal{X}} \varphi_H(p,a|s,\iota) q_H(s,\iota,a) + \sum_{(p,a) \in \mathcal{X}} \varphi_H(p,a|s,\iota) \eta \\
		&= \iota + \eta,
	\end{align*}
	where the last equality holds thanks to the constraint in Equation~\ref{eq:action_promise_constraint} and the fact that $\sum_{(p,a) \in \mathcal{X}} \varphi_H(p,a|s,\iota) = 1$.
	
	Now we consider a time step $h<H$ and assume that the statement holds for $h' = h+1$.
	Then, for every state $s \in \mathcal{S}$, promise $\iota \in I_h(s)$ and couple $(p,a) \in \mathcal{X}$such that $\varphi_H(p,a|s,\iota)>0$ the following holds:
	\begin{align*}
		\qagentpr_h(s,\iota,p,a) &= \sum_{\omega \in \Omega}F_h(\omega|s,a) \left(r^\text{A}_h(s,\omega,p,a) + \sum_{s' \in \sset} P_h(s'|s,w)\vagentpr_{h+1}(s', g_h(s,a,\omega,\iota,s')) \right) \\
		&\ge \sum_{\omega \in \Omega}F_h(\omega|s,a) \left(r^\text{A}_h(s,\omega,p,a) + \sum_{s' \in \sset} P_h(s'|s,w)(g_h(s,a,\omega,\iota,s')-\eta(H-h)) \right) \\
		&\ge q_h(s,\iota,a) - \eta - \sum_{\omega \in \Omega}F_h(\omega|s,a)\sum_{s' \in \sset} P_h(s'|s,w)\eta(H-h) \\
		&=q_h(s,\iota,a) -\eta(H-h+1),
	\end{align*}
	where the first inequality holds by inductive hypothesis, while the second one holds because $\sigma$ is $\eta$-persuasive and $\sum_{\omega \in \Omega}F_h(\omega|s,a)\sum_{s' \in \sset} P_h(s'|s,w) = 1$.
	Finally, we observe that:
	\begin{align*}
		\vagentpr_h(s,\iota) &= \sum_{(p,a) \in \mathcal{X}} \varphi_h(p,a|s,\iota) \qagentpr_h(s,\iota,p,a) \\
		&\ge \sum_{(p,a) \in \mathcal{X}} \varphi_h(p,a|s,\iota) (q_h(s,\iota,a) - \eta(H-h+1)) \\
		&= \sum_{(p,a) \in \mathcal{X}} \varphi_h(p,a|s,\iota) q_h(s,\iota,a) + \sum_{(p,a) \in \mathcal{X}} \varphi_h(p,a|s,\iota) \eta(H-h+1) \\
		&= \iota + \eta(H-h+1),
	\end{align*}
	concluding the proof.
\end{proof}

\promisePersuasive*
\begin{proof}
	Let $\pi$ be the history-dependent policy associated with $\sigma$.
	In order to prove that $\sigma$ (equivalently $\pi$) is $\epsilon$-persuasive, we show that for every step $h \in \mathcal{H}$, history $\tau \in \mathcal{T}_h$ contract $p \in \mathcal{B}$, ad pair of actions $a,a' \in \mathcal{A}$ such that $\pi(p,a|\tau)>0$, the following holds:
	\begin{equation}\label{eq:persuasiveness_to_prove}
		\qagent_h(\tau,p,a) \ge \sum_{\omega \in \Omega}F_h(\omega|s,a') \left(r^\text{A}_h(s,\omega,p,a') + \sum_{s' \in \sset} P_h(s'|s,w)\vagentdev_{h+1}(\tau \oplus (\omega,a,s')) \right) -\epsilon_h,
	\end{equation} 
	where $\epsilon_h = \eta(H-h) \ge \eta H$.
	Thanks to Lemma~\ref{lem:promise_functions_eq}, we have that $\qagent_h(\tau,p,a) = \qagentpr_h(s,\iota^\sigma_\tau,p,a)$, where $s$ is the terminal state of history $\tau$.
	Furthermore the action-value $\qagentpr_h(s,\iota^\sigma_\tau,p,a)$ can be lower bounded as follows:
	\begin{align*}
		\qagentpr_h&(s,\iota^\sigma_\tau,p,a) \\
		&= \sum_{\omega \in \Omega}F_h(\omega|s,a) \left(r^\text{A}_h(s,\omega,p,a) + \sum_{s' \in \sset} P_h(s'|s,w)\vagentpr_{h+1}(s', g_h(s,a,\omega,\iota^\sigma_\tau,s')) \right) \\
		&\ge \sum_{\omega \in \Omega}F_h(\omega|s,a) \left(r^\text{A}_h(s,\omega,p,a) + \sum_{s' \in \sset} P_h(s'|s,w)(g_h(s,a,\omega,\iota^\sigma_\tau,s')-\eta(H-h)) \right) \\
		&\ge \sum_{\omega \in \Omega}F_h(\omega|s,a) \left(r^\text{A}_h(s,\omega,p,a) + \sum_{s' \in \sset} P_h(s'|s,w)\vagentdevpr_{h+1}(s', g_h(s,a,\omega,\iota^\sigma_\tau,s')) \right) -\eta(H-h) \\
		&= \sum_{\omega \in \Omega}F_h(\omega|s,a) \left(r^\text{A}_h(s,\omega,p,a) + \sum_{s' \in \sset} P_h(s'|s,w)\vagentdev_{h+1}(\tau \oplus (\omega,a,s')) \right) -\eta(H-h),
	\end{align*}
	where the first inequality holds by Lemma~\ref{lem:honesty_value}, and the second one thanks to Equation~\ref{eq:promise_persuasive} and the fact that $\sum_{\omega \in \Omega}F_h(\omega|s,a)\sum_{s' \in \sset} P_h(s'|s,w) = 1$.
\end{proof}


\promisingOptimal*
\begin{proof}
	We show that, given an optimal persuasive policy $\pi^\star$, one can always build a promise-form $\sigma = \{\{(I_h,J_h\varphi_h,q_h,g_h)\}_{h \in \mathcal{H}}\}$ that achieves the same expected principal's reward.
%	Observe that $\pi^\star$ does not necessarily implement $\sigma$, since $\pi^\star$ may implement no promise-form policy.
	Given a history-dependent policy $\pi$, we define $\sigma = \sigma_\pi$ as follows:
	\begin{itemize}
		\item $I_h(s) \coloneqq \{\vagent_h(\tau) | \tau = (s_1,a_1,\omega_1, \dots,s_{h-1},a_{h-a},\omega_{h-1},s) \in \mathcal{T}_h\}$ for all $s \in \mathcal{S}$ and $h \in \mathcal{H}$.
		\item $J_h(s) \coloneqq \{\qagent_h(\tau,p,a) | \tau = (s_1,a_1,\omega_1, \dots,s_{h-1},a_{h-a},\omega_{h-1},s) \in \mathcal{T}_h, (p,a) \in \mathcal{X}\}$ for all $s \in \mathcal{S}$ and $h \in \mathcal{H}$.
		\item $\varphi_h(p,a|s,\iota) = \pi(p,a|\tau_{h,s,\iota})$ for all $(p,a) \in \mathcal{X}$, $h \in \mathcal{H}$, $s \in \mathcal{S}$ and $\iota \in I_h(s)$, where:
		\begin{equation*}
			\tau_{h,s,\iota} \in \argmax_{\tau \in \mathcal{T}_h \wedge \text{last}(\tau)=s \wedge \vagent_h(\tau)=\iota } \{\vprincipal_h(\tau)\}
		\end{equation*}
		\item $q_h(s,\iota,a) = \qagent_h(\tau_{h,s,\iota},p^{\pi,\tau_{h,s,\iota},a},a)$, where $p^{\pi,\tau_{h,s,\iota},a}$ is the the single contract $p$ such that $\pi(p,a|\tau_{h,s,\iota})>0$ (which is unique thanks to the revelation principle), or any contract if $\pi(p,a|\tau_{h,s,\iota})=0$ for every contract $p \in \mathcal{B}$.
		We observe that the functions $q_h$ satisfy the constraints represented by Equation~\ref{eq:action_promise_constraint}.
		\item $g_h(s,a,\omega,\iota,s') = \vagent_{h+1}(\tau_{h,s,\iota} \oplus (a,\omega,s'))$ for all $a \in \mathcal{A}$, $h \in \mathcal{H}$, $s,s' \in \mathcal{S}$, $\omega \in \Omega$ and $\iota \in I_h(s)$.
	\end{itemize}
	As a first step, we show that, given that $\pi$ is persuasive, then $\sigma$ is persuasive as well.
	In particular, $\sigma$ is $\eta$-honest with $\eta=0$, since for every $h \in \mathcal{H}$, $s \in \mathcal{S}$, $\iota \in I_h(s)$ and $(p,a) \in \mathcal{X}$ such that $\varphi_h(p,a|s,\iota) = \pi(p,a|\tau_{h,s,\iota})>0$:
	\begin{align*}
		&\sum_{\omega \in \Omega}F_h(\omega|s,a) \left(r^\text{A}_h(s,\omega,p,a) + \sum_{s' \in \sset} P_h(s'|s,w)g_h(s,a,\omega,\iota,s') \right)\\
		&= \sum_{\omega \in \Omega}F_h(\omega|s,a) \left(r^\text{A}_h(s,\omega,p,a) + \sum_{s' \in \sset} P_h(s'|s,w)\vagent_{h+1}(\tau_{h,s,\iota} \oplus (a,\omega,s')) \right) \\
		&= \qagent_h(\tau_{h,s,\iota},p,a) = q_h(s,\iota,a),
	\end{align*}
	where the first equality holds thanks to the definition of $g_h$, the second one due to the definition of $\qagent_h(\tau_{h,s,\iota},p,a)$, and the last equality thanks to the definition of $q_h(s,\iota,a)$.
	Thus, $\sigma$ is $\eta$-honest, with $\eta = 0$.
	
	In order to prove that $\sigma$ is persuasive, we show that Equation~\ref{eq:promise_persuasive} is satisfied and apply Lemma~\ref{lem:promise_persuasive}.
	First, we observe that thanks to the definitions of $\qprincipal_h(\tau_{h,s,\iota},p,a)$ and $g_h(s,a,\omega,\iota,s')$:
	\begin{equation}
		\begin{split}
		\label{eq:promise_form_optimal_rewrite_q}
		\qagent_h&(\tau_{h,s,\iota},p,a) \\
		&= \sum_{\omega \in \Omega}F_h(\omega|s,a) \left(r^\text{A}_h(s,\omega,p,a) + \sum_{s' \in \sset} P_h(s'|s,w)\vagent_{h+1}(\tau_{h,s,\iota} \oplus (a,\omega,s')) \right) \\
		&= \sum_{\omega \in \Omega}F_h(\omega|s,a) \left( r^\text{A}_h(s,\omega,p,a) + \sum_{s' \in \sset} P_h(s'|s,w)g_h(s,a,\omega,\iota,s') \right),
		\end{split}
	\end{equation}
	for every step $h \in \mathcal{H}$, state $s \in \mathcal{S}$, promise $\iota \in I_h(s)$, and action $a \in \mathcal{A}$ with corresponding contract $p \in \mathcal{B}$ such that $\varphi_h(p,a|s,\iota)>0$.
	Furthermore, for every action $\widehat{a} \in \A$:
	\begin{equation}
		\begin{split}
		\label{eq:promise_form_optimal_lower_q}
		\qagent_h&(\tau_{h,s,\iota},p,a) \\
		&\ge \sum_{\omega \in \Omega}F_h(\omega|s,\widehat{a}) \left( r^\text{A}_h(s,\omega,p,\widehat{a}) + \sum_{s' \in \sset} P_h(s'|s,w)\vagentdev_{h+1}(\tau_{h,s,\iota} \oplus (a,\omega,s')) \right) \\
		&= \sum_{\omega \in \Omega}F_h(\omega|s,\widehat{a}) \left( r^\text{A}_h(s,\omega,p,\widehat{a}) + \sum_{s' \in \sset} P_h(s'|s,w)\vagentdevpr_{h+1}(s',g_h(s,a,\omega,\iota,s')) \right),
		\end{split}
	\end{equation}
	since $\pi$ is persuasive and, thanks to Lemma~\ref{lem:promise_functions_eq}, $\vagentdev_{h+1}(\tau_{h,s,\iota} \oplus (a,\omega,s')) = \vagentdevpr_{h+1}(s',g_h(s,a,\omega,\iota,s'))$.
	As a result, by combining Equation~\ref{eq:promise_form_optimal_rewrite_q} and Equation~\ref{eq:promise_form_optimal_lower_q}, we have that Equation~\ref{eq:promise_persuasive} is satisfied. 
	Consequently, by applying Lemma~\ref{lem:promise_persuasive}, the policy $\sigma$ is persuasive.
	
	In order to conclude the proof, we show that the promise-form policy $\sigma$ achieves at least a principal's expected cumulative reward as good as that obtained by $\pi$.
	This implies that the promise-form policy $\sigma^\star = \sigma^\star_{\pi^\star}$, where $\pi^\star$ is an optimal history dependent policy, is optimal.
	Let $\pi^\sigma$ be the history-dependent policy that implements $\sigma$ according to Algorithm~\ref{alg:implement} (observe that it may be different from $\pi$).
	Formally, we prove by induction over $h \in \mathcal{H}$ that $V^{\text{P},\pi^\sigma}_h(\tau) \ge \vprincipal_h(\tau)$ for every step $h \in \mathcal{H}$ and history $\tau \in \mathcal{T}_h$.
	As a base case, we consider $h=H$. 
	For every history $\tau \in \mathcal{T}_H$ ending in state $s$ it holds that:
	\begin{align*}
		\vprincipal_H(\tau) &\le \vprincipal_H(\tau_{H,s,\iota^\sigma_\tau}) \\
		&=\sum_{(p,a) \in \mathcal{X}} \pi(p,a|\tau_{H,s,\iota^\sigma_\tau}) \sum_{\omega \in \Omega} F_H(\omega|s,a) r^P_H(s,\omega,p) \\
		&= \sum_{(p,a) \in \mathcal{X}} \varphi_H(p,a|s,\iota^\sigma_\tau) \sum_{\omega \in \Omega} F_H(\omega|s,a) r^P_H(s,\omega,p) \\
		&= \vprincipalpr_H(s,\iota^\sigma_\tau) \\
		&= V^{\text{P},\pi^\sigma}_h(\tau),
	\end{align*}
	where the inequality holds due to the definition of $\tau_{H,s,\iota^\sigma_\tau}$ and the last equality one thanks to Lemma~\ref{lem:promise_functions_eq}.
	
	Now we consider $h < H$ and assume that the statement holds for $h' = h+1$.
	Then for every history $\tau \in \mathcal{T}_h$ ending in some state $s \in \mathcal{S}$ the following holds:
	\begin{align*}
		\vprincipal_h(\tau) &\le \vprincipal_h(\tau_{h,s,\iota^\sigma_\tau}) \\
		&=\sum_{(p,a) \in \mathcal{X}} \pi(p,a|\tau_{h,s,\iota^\sigma_\tau}) \qprincipal_h(\tau_{h,s,\iota^\sigma_\tau},p,a) \\
		&=\sum_{(p,a) \in \mathcal{X}} \varphi_h(p,a|s,\iota^\sigma_\tau) \qprincipal_h(\tau_{h,s,\iota^\sigma_\tau},p,a),
		\label{eq:promise_form_optimal_proof_vprincipal}
	\end{align*}
	where the inequality holds due to the definition of $\tau_{H,s,\iota^\sigma_\tau}$.
	Furthermore, for every contract $p \in \mathcal{B}$ and action $a \in \A$ it holds that:
	\begin{align}
		\qprincipal_h&(\tau_{h,s,\iota^\sigma_\tau},p,a) \\
		&= \sum_{\omega \in \Omega}F_h(\omega|s,a) \left( r^\text{P}_h(s,\omega,p) + \sum_{s' \in \sset} P_h(s'|s,w)\vprincipal_{h+1}(\tau_{h,s,\iota^\sigma_\tau} \oplus (a,\omega,s')) \right) \\
		&= \sum_{\omega \in \Omega}F_h(\omega|s,a) \left( r^\text{P}_h(s,\omega,p) + \sum_{s' \in \sset} P_h(s'|s,w)g_h(s,a,\omega,\iota^\sigma_\tau,s') \right) \label{eq:promise_form_optimal_1}\\
		&\le \sum_{\omega \in \Omega}F_h(\omega|s,a) \left( r^\text{P}_h(s,\omega,p) + \sum_{s' \in \sset} P_h(s'|s,w)\vprincipal_{h+1}(\tau_{h+1,s',g_h(s,a,\omega,\iota^\sigma_\tau,s')}) \right) \label{eq:promise_form_optimal_2}\\
		&\le \sum_{\omega \in \Omega}F_h(\omega|s,a) \left( r^\text{P}_h(s,\omega,p) + \sum_{s' \in \sset} P_h(s'|s,w) V^{\text{P},\pi^\sigma}_{h+1}(\tau_{h+1,s',g_h(s,a,\omega,\iota^\sigma_\tau,s')}) \right) \label{eq:promise_form_optimal_3}\\
		&\le \sum_{\omega \in \Omega}F_h(\omega|s,a) \left( r^\text{P}_h(s,\omega,p) + \sum_{s' \in \sset} P_h(s'|s,w)\vprincipalpr_{h+1}(s',g_h(s,a,\omega,\iota^\sigma_\tau,s')) \right) \label{eq:promise_form_optimal_4}\\
		&= \qprincipalpr_h(s,\iota^\sigma_\tau) \\
	\end{align}
	where Equation~\ref{eq:promise_form_optimal_1} holds hanks to the definition of $g_h(s,a,\omega,\iota^\sigma_\tau,s')$, Equation~\ref{eq:promise_form_optimal_2} thanks to the definition of $\tau_{h+1,s',g_h(s,a,\omega,\iota^\omega_\tau,s')}$, Equation~\ref{eq:promise_form_optimal_3} holds by induction, while Equation~\ref{eq:promise_form_optimal_4} is verified according to Lemma~\ref{lem:promise_functions_eq}.
	Thus, by combining this result with Equation~\ref{eq:promise_form_optimal_proof_vprincipal} we get:
	\begin{equation*}
		\vprincipal_h(\tau) \le \sum_{(p,a) \in \mathcal{X}} \varphi_h(p,a|s,\iota^\sigma_\tau) \qprincipalpr_h(s,\iota^\sigma_\tau) =\vprincipalpr_h(s,\iota^\sigma_\tau) = V^{\text{P},\pi^\sigma}_h(\tau),
	\end{equation*}
	where the last equality holds thanks to Lemma~\ref{lem:promise_functions_eq} and the definition of $\iota^\sigma_\tau$, concluding the proof.
\end{proof}
